# Supplementary material for: A Feature-based Classification of Model Repair Approaches
Source: arXiv:1504.03947 source file (2015-04-15)
Supplement: Supplementary file 1 [file appendices.tex]

\appendices
%\begin{bibunit}[IEEEtran]
%\begin{bibunit}[abbrv]

\section{Techniques Overview}
\nuno{Dummy section to store technique information without cluttering the main text.}

\subsection{Not addressed in the main text}

 \cite{KortgenN:11}
  
 \cite{KozlenkovZ:04} uses prolog to generate fixes
 
 \subsubsection{Repair Dependence Graph} 
 \label{sec:rinard}

 \cite{DemskyR:05} present a model-based approach to data structure repair, a technique for enabling programs to execute successfully in the presence of otherwise fatal data structure corruption errors. The method involves two views: a concrete view of the data structures as they are represented in the memory and an abstract view that models the data structures as sets of objects and relations between objects.

 A set of model definition rules, encapsulating the data structure representation complexity, translates the concrete data structures to the sets and relations in the abstract model. The key consistency constraints are then expressed using the sets and relations in this model, defining important data structure consistency properties.

 An automatically generated repair algorithm finds and repairs any data structures that violate the defined consistency properties. These violations are repaired by automatically translating model repairs back through the model definition rules to automatically derive a set of data structure updates that implement the repair. The compiler uses goal-directed reasoning to statically map these model repair actions to data structure updates.

 A repair dependence graph is used to capture dependencies between consistency constraints, repair actions, and the abstract model. Supporting formal reasoning about the effect of repairs on both the model and the data structures, this graph presents a set of conditions that identify a class of cycles whose absence guarantees that all repairs will successfully terminate. An algorithm then removes nodes in the graph to eliminate problematic cycles, preventing the repair procedure from choosing repair strategies that may not terminate.
 
 \subsubsection{Main Remarks}
 \label{ss:mremarks}

 Although the approach from \cite{XiongHZSTM:09} repairs models automatically, the user has to manually specify the fixing behavior, an error-prone approach without guarantees of completeness. In \cite{PuissantSM:13}, once the resolution plan is generated, the user must replace temporary elements by concrete elements, so
 this is not a fully automatic approach. However, no fixing annotations need to be manually specified, and users can adapt the order in which resolution plans are presented by assigning different costs to edit operations.

 In \cite{DemskyR:05}, a repair dependence graph is used to capture dependencies and resolve side effects. However, it is not incremental nor evaluates models without the need to translate them to an abstract representation.

 Among all approaches, the one from \cite{RederE:12} appears to be the one which scales better, since it is iterative, evaluates models directly, does not necessarily repair all inconsistencies at once, and follows a syntactic-based analysis.
 However, the approach is not fully automatic as the user must instantiate proposed repairs, does not follow the \textit{least-change} principle and no control over repairs generation is given.

 Although less scalable when compared to Egyed's approach, the one from \cite{MacedoGC:13} is fully automatic, generating repaired models which are as close as possible to the original, and provides control over repairs generation through the specification of allowed edit operations.
 Straeten's technique \cite{StraetenPM:11} does not ensure
 minimality of the repairs nor control over its generation.

 \begin{table}[t]
   \begin{tabular}{  r | c | c | c | c | c | c | c | c | c | c | c } 
     & \rotatebox{90}{incremental} & \rotatebox{90}{user can choose repairs} & \rotatebox{90}{repairs automatically applied} & \rotatebox{90}{complete} & \rotatebox{90}{no manually specified repairs} & \rotatebox{90}{one inconsistency at a time} & \rotatebox{90}{side effects handling} & \rotatebox{90}{principle of \textit{least-change}} & \rotatebox{90}{control over repair generation} & \rotatebox{90}{syntactic-based}\\ \hline

   \cite{XiongHZSTM:09} & & & \checkmark & \xmark & \xmark & & & \xmark & \checkmark & \checkmark  \\ \hline
   \cite{PuissantSM:13} & & \checkmark & \xmark  & \checkmark & \checkmark & \xmark  & & \xmark & \checkmark & \xmark \\ \hline
   \cite{StraetenPM:11} & \xmark &  & \checkmark & \checkmark & \checkmark & \checkmark & \checkmark & \xmark & \xmark & \xmark \\ \hline
   \cite{RederE:12} & \checkmark & \checkmark & \xmark & \checkmark & \checkmark & \checkmark & \checkmark & \xmark & \xmark & \checkmark  \\ \hline
   \cite{MacedoGC:13} & \xmark & \checkmark & \checkmark & \checkmark & \checkmark & \xmark & \checkmark & \checkmark & \checkmark & \xmark \\ \hline
   \cite{DemskyR:05} & \xmark &  & \checkmark &  & \checkmark & \xmark & \checkmark & \xmark & \checkmark & \checkmark  \\ \hline

   \end{tabular}
   \caption{Comparison of approaches to model repair.}
   \label{tab:comparison}
 \end{table}
 
 \subsection{Not model repair but may be relevant}
 
    \subsubsection{motivation} 
    
    consistency management~\cite{FinkelsteinGHKN:94,NuseibehER:00}
    
    tolerating inconsistencies~\cite{}

    model evolution~\cite{Mens:08}
    
    kinds of relationships between models~\cite{KolovosPP:08}
    
    survey of incremental TGG techniques, thus suitable for model synchronization~\cite{LeblebiciASHRG:14}
    
    nice survey/classification of model repair techniques~\cite{SchoenboeckKEKSWW:14}

    design space for (pairwise) synchronization~\cite{AntkiewiczC:07}

    \cite{BrancoXCKV:14} a case study on consistency management over BPM that concluded that repair proposal should act in an online setting
    
 \subsubsection{feature models} \cite{Lopez-HerrejonE:12} proposes fixing configurations by mapping model elements to features and defining consistency at feature model level (not directly related to this survey, but maybe worth mentioning)
 
 \cite{HwanKC:05} proposes a technique to keep feature models consistent with configurations through traceabilities; has a neat overview of model synchronization systems.

 \subsubsection{consistency checkers} \cite{BiehlL:09,MalgouyresM:06,QueraltT:06,CabotT:09,Egyed:06,RederE:13} only check for consistency of UML (do not fix) but that might be important to cite (\cite{CabotT:09,Egyed:06} are incremental)
 
 \cite{EngelsHK:01,TsiolakisE:00} for checking consistency of UML diagrams only; from \cite{GieseW:09} ``Another category of approaches detects the consistency between two models. However, these approaches are specialized on particular model types.''
 
 \cite{LucasMA:09} is an in-depth survey on UML consistency management, but does not explore repair functionalities; classifies formalism and deployment features.
  
  \cite{BlancMMM:08}
  
 \subsubsection{change impact analysis} \cite{KellerSD:09} support inconsistency resolution through change impact analysis: based on the meta-model, they calculate related meta-classes; then when a concrete model element is updated, that relationship is used to retrieve other impacted elements; \cite{BriandLOS:06}, given a set of rules, proposes algorithms that, given a model update, return a set of possibly affected elements (between different UML models); \cite{SpanoudakisK:02};

 \subsubsection{others} \cite{MensS:06} appears to be an extension to \cite{MensSD:06} with some completeness analyzing about constraint definition, repair operations and resolution rules.

 \cite{EtzlstorferKKLRSSW:13} incremental model transformation
 
 \cite{GreenyerK:07} does not actually propose a technique, rather just compares TGGs with QVT
 
 \cite{NohrerRE:11} propose to handle clusters of overlapping consistencies to improve efficiency; preliminary work, argues that finding elements that cause multiple inconsistencies may improve the performance of the technique.

 \cite{FinkelsteinKNFG:92} ViewPoints

 \subsubsection{constraint repair}
 \cite{LamsweerdeDL:98} supports temporal logic, focuses on requirements engineering. most presented techniques relax the goals (i.e., the constraints) rather than the models.
 
 \cite{DemuthLE:12b} propose the definition of constraint templates that are instantiated as the meta-mode evolved to concrete constraints.

 \subsubsection{meta-model co-evolution}
 
 meta-model co-evolution is related to model repair, but opens a whole new world of research (model migration!). select some that seem more connected to model repair. e.g. \cite{SchoenboeckKEKSWW:14} is pure model repair, as the original meta-model is disregarded.
 
 \cite{GruschkoKP:07} reasons about the evolution of meta-models; first, changes in the meta-model are detected (either state-based and infer delta, or delta directly); then a transformation (ATL/ETL) is defined that maps elements from the original meta-model to the updated (deltas are ignored!).

 \cite{CicchettiREP:08}
 
 \cite{RoseHWKGPP:10} survey

 \cite{Herrmannsdoerfer:10}
 
 \subsubsection{correct evolution}

 \cite{HegedusHRBV:11} has related work on this: ``model construction deals with creating consistent models through a series of operations''.
 
 \cite{NuseibehER:00} argues that this is not desirable as it forces models to be consistent at all time;
 
 \cite{GuerraL:04} not really model repair, but more correct evolution. to manage the consistency between abstract and concrete models (in particular, in visual languages); they use event-driven TGGs to map actions in the concrete model back to the abstract one; each event introduces an event node, which is then processed by graph transformation rules. from~\cite{GieseW:09} ``The incremental transformation approach in the multi-paradigm modeling tool AToM3 is triggered by user actions like creating, editing, or deleting elements. However, this requires the specification of all possible user actions and appropriate activities for the updates. Although the specification is done visually using graph grammar based techniques and is therefore more appropriate than ad-hoc programming, the required specification effort increases with the number and granularity of the available user actions. Due to this operational characteristic, the overall consistency of the approach is difficult to guarantee. In addition, a complete model transformation from scratch is not supported.''

 \cite{HaesenS:04} proposes a framework for the correct development of UML models: every user update is (to some extent) guaranteed to be consistent (consistency by monitoring, consistency by construction, consistency by analysis).

 \cite{EngelsHKG:02} extends \cite{EngelsKHG:02} regarding correct evolution of UML-RT models;

 \paragraph{model-code synchronization} \cite{BottoniPPT:08}

 \paragraph{implicit consistency notion}
 
 every BX not based on the notion of consistency relation (lenses and company)
 
  \cite{HearndenLR:06} incremental model transformation from a source model to a target model (aka BX); the specification artifact is the transformation, no actual notion of consistency; from \cite{GieseW:09} ``extend a declarative logic-based transformation engine in order to incrementally synchronize a target model with source model changes. The presented approach records a transformation execution and maps changes in the source model to the execution record. This enables the calculation of necessary updates of the target model in order to keep both models consistent to each other. The solution comes at the cost of a permanently maintained transformation execution context. For large transformations further optimizations of the extra needed space for the execution context have to be considered. In addition, it is not clear whether a bidirectional synchronization can be executed on the same execution record or if one execution record for each transformation direction is needed. However, utilizing model transformations for synchronization purposes is quite obvious and seems to be a promising approach.''  

  \paragraph{batch transformation} these approaches focus on creating a target model from a source model, but are not able to restore the consistency between two existing models (typically, TGGs!)
  
  \cite{Konigs:09} proposes the deployment of QVT as TGGs so that the technique is standard compliant

 \subsection{Addressed in the main text}

 in \cite{MafaziMS:14} there is a `reference model' and a set of `views', as well as a (many-to-one) mapping from reference elements to view elements; updates on the view are merged in the reference model and then propagated back to the views. this is done by detecting the updates on the views and using the mapping to reflect them on the reference model. 
 
 \cite{SchoenboeckKEKSWW:14} is based on ASP; the problem's constraints arise from the meta-model (structural), additional constraints (OCL) and any other defined by the user; it is rule-based: for each inconsistency, there is a defined set of actions; however, it is also solver-based, which is used to apply the rules until consistent solutions are reached; it is complete, returns all consistent solutions, and provides a rank: by default, calculates structural similarities, but the user may define additional criteria. has a survey comparing model repair approaches~\cite{SilvaMBB:10,BlancMMM:08,EgyedLF:08,EramoPRV:08,Herrmannsdoerfer:10,Kortgen:10,MensSD:06,NentwichEF:03,PuissantMS:10,StraetenMSJ:03,XiongHZSTM:09}.

 \cite{KolovosPP:08} advocates the use of Epsilon Validation Language (EVL) to generate fixes; EVL is part of the Epsilon Object Language (EOL)~\cite{}, that extends OCL with multi-model constructs; EVL also allows the definition of ``fix'' operations that provide alternatives to fix constraints.

 \cite{SilvaMBB:10} is built on Praxis, where models are defined by edit operations; for each inconsistency, the system calculates a set elements that are expected to have caused the inconsistency; then, a set of user-defined rules specifies potential fixes for each problematic element. since models are created by edit operations, the system prioritizes fixing the most recent elements (where does this fit in the features?); it also user a search algorithm to search for repairs with a minimal number of operations (least-change?).

 \cite{SpanoudakisZ:01} is a famous (and old) survey on consistency management. Regarding inconsistency fixing, analyzes \cite{Easterbrook:91,RobinsonF:94,EasterbrookN:96,SpanoudakisF:97,LamsweerdeDL:98,NuseibehR:99} (from the 90s) (from \cite{KusterR:07}, `they concluded that the most important open research issue in inconsistency handling is providing more guidance to the user for choosing among multiple alternative resolutions. The authors argue that resolutions should be ordered based on cost, risk and benefit. They further conclude that existing approaches do not adequately address efficiency and scalability of inconsistency detection in models that change during the resolution process. In our approach, we use side-effects and costs for evaluating alternative resolution and avoid rechecking the whole model after a resolution is applied'). 
 
 \cite{Easterbrook:91} seems to be the first study on inconsistency resolution; it is an informal approach, where the users informally point conflicting elements (exploring phase), propose abstract repairs (generative phase) and finally select the best suited one (evolution phase); fully interactive, allows the users to annotate extra information and importances to conflicts (education and negotiation); based on a lightweight version of viewpoints. No actual support to specify constraints: users simply flag conflicting elements.
 
 \cite{EasterbrookN:96} is based on the viewpoint framework, stakeholder defines rules and resolutions, which are selected by the user; motivation for why inconsistencies appear. 
 
 \cite{SpanoudakisF:97} is also based on viewpoints, tries to find an isomorphism that minimizes the distance between two object-oriented models; the user then suggests modifications to the isomorphism, and repair actions are proposed that render that modified isomorphism the minimal one. not really least-change: distance function is used to calculate the isomorphism; when the user repairs the isomorphism, modifications that render that the minimal one are proposed (which is not necessarily a least-change o models.)
 
 \cite{NuseibehR:99} uses abduction over QC logic to restore consistency. constraints are defined as propositional formulas (?); once a consistency is detected, the causes for the existence of the inconsistent literals is searched; this is possible because constraints are simply implications; repairs are simply suggestions for the deletion of literals. (extends ~\cite{HunterN:98}, which was rule-based like~\cite{FinkelsteinGHKN:94}).
 
 \cite{FinkelsteinGHKN:94} seminal work on consistency management in ViewPoints. temporal rule-based.

 \cite{Kortgen:10} proposes a technique to manage the consistency between decoupled models (heterogeneous environments, thus state-based). it is based on TGGs. focuses on handling inconsistencies where the traceability was rendered inconsistent (as opposed to inconsistencies caused by unlined elements, which can be solved simply by applying the rules) (\cite{GieseW:09} also handled these).
 
 \cite{EgyedLF:08} build up on \cite{Egyed:07}, and is essentially based on the instantaneous consistency checker from \cite{Egyed:06}: the checker uses the constraint instantiations to detect every affected element that is a possible location to fix~\cite{Egyed:07}; then, once the user selects an element, rules defined for each type of element are applied~\cite{EgyedLF:08}; before being presented to the user, the checker is run again so that those that cause negative side effects are removed. to have a limited set of solutions, rules only consider elements already present in the initial model (bounded). from \cite{DamW:10} ``proposes a mechanism for fixing inconsistencies in UML design models by automatically generating a set of concrete changes. Their approach uses pre-defined choice generation functions, which compute possible values for locations in the model, for instance, possible new names for a method. The generated options are checked against the constraints and are rejected if they do not in fact repair the constraint, or if they cause new constraint violations. However, this work has several major limitations. Firstly, they consider only a single change at a time, and consequently do not take into account the cases where a single change may not resolve all inconsistencies, or may even temporarily introduce new ones before reaching a consistent state. Secondly, the choice generation functions are written by hand, and may not be complete, meaning that the approach is incomplete: it only considers a subset of the possible ways of repairing a given constraint violation. Finally, their approach does not consider the creation of model elements, which in our opinion is an important part of change propagation.''
 
 \cite{AmelunxenLSS:07} is another rule-based approach. uses the FUJABA + MOFLON framework to check and repair the consistency of MATLAB simulink models; advocates that OCL and pattern matching is not expressive enough to specify consistency; uses snippets of imperative code (supported by FUJABA).
 
 \cite{EndersHGTT:02} interprets the ViewPoints framework as distributed graph transformations; essentially TGGs (the term had not been coined yet); graph rules are used to check intra- and inter-view consistency and to repair inconsistencies through pattern matching. links are created manually by the user from traceability rules. from \cite{BeckerHLW:07} ``a consistency management approach for different view points of development processes is presented. The formalism of distributed graph transformations is used to model view points and their interrelations, especially consistency checks and repair actions. To the best of our knowledge, this approach works incrementally but does not support detection of conflicting rules and user interaction.'' 
 
 \cite{WagnerGN:03} presents the overall architecture of FUJABA. incremental (in the sense that updates are operation-based) graph transformations; detection rules and resolution rules; resolution rules are applied in runtime to check for conflicts. from \cite{KusterR:07}: ``The FUJABA tool suite supports both manual and automatic incremental inconsistency resolution. Consistency checking rules can be configured by the user and organized into different categories in order to support domain- or project-specific consistency requirements. Consistency checking rules and inconsistency resolution rules are specified using graph grammar rules and executed by a FUJABA rule engine. Although different categories could also be used for obtaining different priorities, our approach can be seen as complementary because we focus on the evaluation of several alternative resolutions for one inconsistency based on side-effects and costs''; from \cite{BlancMMM:08} ``The framework monitors change events and tries to match them against detection rules that are defined as graph grammar patterns. If a match is detected then the rule is automatically re-checked. Wagner does not provide any performance analysis and does not ensure that his approach is scalable. Indeed, Wagner indicates that rules should not be time consuming in order to not block the user while he is building his models'' \cite{WagnerGN:03,HaesenS:04} from \cite{DamWP:06} ``the event-driven consistency check approaches make an improvement in terms of efficiency by incrementally re-validating only the context of the last changes and not the whole model''. Checks for negative side-effects: every repair plan is executed prior to being presented to the user and checked for newly introduced inconsistencies.
 
 \cite{HausmannHS:02} is also based on graph transformations, and assumes the existence of traceability links between elements; analysis some properties of these links; once inconsistencies are detected, proposes some abstract ways to handle them (delete the elements, create dummy (abstract) elements, create warning and let user act); element-level links are created by the consistency restoring rules.

 \cite{KonigsS:06} extends \cite{KonigsS:05} generalize TGGs to handle multiple domains; the example is a quadruple graph grammar. from \cite{BeckerHLW:07} ``triple graph grammars are generalized to handle integration of multiple documents rather than pairs of documents. From a single synchronous rule, multiple rules are derived in an analogous way as in the original TGG approach. The decomposition into multiple steps such as link creation, context check, and rule application is not considered.''

 \cite{LiuEM:02} is a rule-based approach to managing intra- and inter- (through pattern matching) model consistency of UML diagrams. detection rules introduce inconsistency elements (with location and rule identification); resolution rules act on identification of those elements (may exist multiple for each inconsistency); cleanup rules remove spurious elements; when more than one rule can be applied, `conflict set resolution' selects on that has higher priority. from \cite{MensS:06} ``a logic rule-based approach (as opposed to a graph-based one) is proposed to detect and resolve inconsistencies in UML models, using the Java Rule Engine JESS. The architecture of this tool provides a Rule Engine Abstraction Layer, making it possible to replace their rule engine by a graph-based one''. review of kinds of causes for inconsistencies (due to redundancy, standard conformity or change). 

 \cite{IvkovicK:04} requires the user to map the models, meta-models, traceabilities and repair operations into graph concepts. the user then defines a mapping between edit operations between both models. if such mapping does not restore consistency, the procedure fails; from \cite{GieseW:09} ``developed an approach for model synchronization that is based on implicit traceability relations, i.e., the relations are defined and encoded between the meta-models rather than the interrelated models. In their approach, special graphs for the purpose of model synchronization have to be derived from the meta-models. In addition, respective modifications represented as atomic graph operations on nodes and edges (e.g., insert, delete, modify) have to be specified and implemented. In order to synchronize two models, the operations applied to the source model are traced and transformed according to operations for the target model. Then, the transformed operations are executed on the target model. In a final step, an equivalence relation checks whether the synchronization was executed successfully. For the definition of a model synchronization between two models seven steps have to be accomplished. This is too complex if customizations of the model synchronization should be allowed to end users. Moreover, the authors agree that in practice implicit model synchronization will not suit all synchronization scenarios.''
 
 \cite{RederE:10} is the implementation of Egyed's technique

 more TGGs from \cite{KusterR:07}: ``Work on incremental transformations TGGs studies the problem of keeping two models synchronized (\cite{GieseW:09} extends \cite{GieseW:06}, \cite{BeckerHLW:07} extends \cite{BeckerLW:04}). This is achieved by analyzing changes in one model and applying incremental updates for re-establishing consistency. Although these updates are analyzed for conflicts, a detailed evaluation of side-effects is not addressed''. TGG productions are monotonic and cannot delete elements: deletion is achieve artificially by checking for inconsistent links~\cite{BeckerHLW:07,GieseW:09}. \cite{BeckerHLW:07} also performs conflict analysis when choosing which production to apply, which the user has to select.

 \cite{PuissantSM:13} extends \cite{PuissantSM:12}

 \cite{PuissantMS:10} is the initial work for \cite{PuissantSM:13}, where forward planning is used instead of regression planning.

 \cite{GieseW:09} follows a `generative' approach: models are consistent if it is possible to generate them from the defined graph transformations; when models are initially generated, a traceability between them is calculated and stored; then, when one of them is update, this information is used to achieve an incremental algorithm, that does not required the batch generation of the models. built over FUJABA. (good biblio). can fix inconsistencies caused by deletion and modification in the following way: once an inconsistent link is found, if it is due to inconsistent attributes, they are propagated; if it is due to failed pattern matching, the link is removed; the elements are now considered fresh, and new rules will be applied that will fix the inconsistency by modifying the target graph.
 
 \cite{DamW:10} proposes repair plans for change propagation on UML, considers all inconsistencies at once, constraints defined specifically in OCL; much like Egyed's, it generates repairs from OCL constraints, which the authors guarantee to be correct and complete; operations are creation, deletion, connection, disconnection, or modification of model elements; then they calculate costs for each repair, taking into consideration that other constraints may be introduced or removed; the user is presented with the cheapest. essentially, the application of \cite{DamW:11} to UML models (rather than agent-oriented models).

 \cite{DamW:11} extends both \cite{DamW:07} and \cite{DamWP:06} (good biblio). they propose a technique for change propagation in agent-oriented models. \cite{DamWP:06} was the initial approach; constraints and repair plans seem to be hard-coded.

 \cite{DamW:07} builds up on  \cite{DamWP:06} by automatically deriving repair plans from OCL constraint; architecture appears to be very similar to \cite{DamW:10}. `` We recognize that fixing one violated constraint may also repair or violate others as a side effect, and so the cost calculation algorithm computes the cost of a given repair plan instance as including the cost of its actions (using basic costs assigned by the repair administrator), the cost of any other plans that it invokes directly, and also the cost of fixing any constraints that are made false by executing the repair plan. If there are several equal least cost plans, they are presented to the user, otherwise the cheapest plan is selected. Once a plan is selected, it is then executed to fix the violation, and hence propagate changes. We allow the repair administrator to specify the repair cost for each basic repair action. The repair administrator may use this mechanism to adjust the change propagation process''; they also claim that ``Our translation schema guarantees completeness and correctness, i.e. there are no repair plans to fix a violation of a constraint other than those produced by the generator; and any of the repair plans produced by the generator can fix a violation. However, we also allow the repair administrator to use their domain knowledge and expertise to modify generated repair plans or remove plans that should not be executed. In section 4 we discuss this in more detail''. OCL language is only logical (no equality!); side-effects are handled by assigning costs to fixing other inconsistencies; repairs may be `creates', which are abstract; repair administrator may disable or modify plans; abstract repair plans are are generated at static time from constraints, being instantiated in run-time for concrete models; some repairs (e.g., creation) may need user input. as far as I can understand, this is least-change: they search all possible repair plans for the cheapest.
 
 \cite{DamLG:10} adapts \cite{DamW:08,DamWP:06,DamW:07} to the Enterprise Architectures setting, using Alloy underneath.

 \cite{MensSD:06}  analysis dependencies between rules to avoid side effects at static time (no models); inconsistency detection is performed through graph transformations that introduce `inconsistency' nodes; resolutions is performed through resolution rules over such nodes;  (from \cite{KusterR:07}, `it uses the AGG graph transformation tool to detect potential dependencies between different inconsistency resolutions. Inconsistency detection and resolution rules are expressed as graph transformation rules in AGG and are then analyzed using critical pair analysis. Analysis results point to potentially conflicting resolutions, resolutions that may induce or expire other types of inconsistencies and potential cycles between resolutions.').

 \cite{KusterR:07} requires each inconsistency to be annotated with costs and resolutions with consequent (positive and negative) side-effects; this allows the user to assess the impact of choosing a resolution; the running example is of synchronization of state diagrams with activity diagrams. Detected inconsistencies refer to the broken constraint and the involved elements (good biblio).
 
 \cite{DamG:14} proposes an abstract framework for minimal change propagation, so that a single repair is selected from among all well-formed ones. they also propose that operations be attached with weights to be minimized.
 
 \cite{NentwichEF:03} for arbitrary XML (built over xlinkit \cite{NentwichCEF:02}). repairs are automatically derived from first-order logic XPath constraint; the user can then disable some of these rules; these are then instantiated for inconsistent models (from \cite{KusterR:07}, ``they propose to generate inconsistency resolutions (called repair actions) automatically from consistency constraints that are specified in first order logic. As opposed to our approach, generated repair actions do not take into account a concrete model violating consistency constraints and also do not consider side-effects.'').
 
 from \cite{RederE:12} ``their \cite{NentwichEF:03} approach is conservative and may suggest non-minimal and even incorrect repair actions if the design rule is partially violated only. Nonetheless, we consider this work as a foundation to our work. Table 1 is clearly based on their principles.''
 
  from \cite{DamW:11} `` The basic idea behind the rules is that each constraint is analysed, and all possible ways of repairing it are generated. This basic idea was previously proposed by Nentwich et al. \cite{NentwichEF:03} who derived repair actions from constraints. However, although the basic principle of deriving repair options from constraints is the same, there are significant differences in the details. Firstly, and most importantly, our work deals with the repair of multiple constraints which can interact (e.g. repairing one constraint can also, as a side-effect, repair another constraint). Secondly, we use a richer representation for repair plans. Finally, our constraints are in a richer language, which is an industry standard (OCL). For instance, xlinkit does not support set expressions that result in new sets. On the contrary, OCL provides a wide range of such operations on a set such as returning a subset of a set that contains elements for which a given constraint holds or does not hold (select and reject), or returning a set containing all the elements that are either in one set or the other but not in both (symmetricDi f f erence), or returning a union or intersection of two sets (i.e. union and intersection). OCL also provides an if–then–else expression which is not supported in xlinkit. Furthermore, unlike xlinkit, OCL supports not only sets but also other types such as bags and sequences.''

 from \cite{XiongHZSTM:09} ``Some approaches seek for automated means to generate a set of fixing actions from logical expressions. Typical approach includes the white-box analysis of first-order logic \cite{NentwichEF:03} and the black-box analysis of the consistency rules \cite{EgyedLF:08}. Compared to ours, these approaches generate the fixing actions purely from a consistency relation, but require human interventions in executing the actions, by specifying some locations to fix, choosing one among a set of actions or filling some missed parameters. We believe both types of approaches are important to consistency management, because while some consistency relations are suitable to be established all the time through automatic fixing, some consistency relations are suitable to be manually resolved by humans.''

 from \cite{BrancoXCKV:14} ``fixing plans for given actions in the model sequence. In \cite{NentwichEF:03}, Nentwich et al describe a framework for repairing inconsistent documents in a distributed setting. Their approach consists of defining a mapping from the logical language used to describe the inconsistency rules into a set of repair actions that, after being executed, will make the model consistent again. In \cite{MensSD:06}, Mens et al present an approach for consistency management on top of graph transformation tool AGG. They detect the inconsistencies in the model by the means of the inconsistency detection rules (that tags model elements as conflicted) and fix inconsistencies by the means of the resolution rules (for each possible resolution of every kind of inconsistency there is one rule that describe how should be the model after fixed). They use then a critical pair analysis algorithm to infer dependencies between rules and aid the user in the task of fixing the model. Both approaches automate the process of defining how to deal with the inconsistency by proposing a set of actions that fix each of them, and they automate the definition of what are the impacts of the suggested repairs: they detect inconsistencies among different plans and thus discourage their application at the same time. However, the decision on the order of the execution of the proposed repair actions (or plans) is left to the user. In our proposal, we cope with this problem by exploring the set of generated choices and actually delivering a plan of execution of the proposed actions.''
 
 \cite{StraetenMSJ:03} is initial work on using description logic to manage consistency; is a purely rule-based I approach: rules are defined that fix the (DL representation) of the model; a single rule is applied at a time, so a single inconsistency is fixed (although it possibly fixes multiple instances of the same inconsistency?); the meta-model is UML and is fixed (embedded in the DL representation); the translation between UML models and DL is manual; the rules are also hard-coded; the UML meta-model is extended with traceability elements, so it is also able to manage inter-model consistency.
 
 \cite{MensSS:05} extends \cite{StraetenMSJ:03} and \cite{SimmondsSJM:04}; good definitions of consistency management and types of inconsistencies. extend the UML meta-model to accommodate version control and horizontal/vertical traces; everything is translated to description logic (as expressible as 2 variable fragment of FOL) and repairs are rule-based. 
 
 \cite{StraetenD:06} builds on \cite{StraetenMSJ:03,SimmondsSJM:04,MensSS:05} and applies it to model refactoring. it is a rule based approach: instead of defining constraints, one defines rules that are triggered when inconsistencies occur.
 
 \cite{GrundyHM:98} more multi-view consistency; rather abstract; more motivation on tolerating inconsistencies.
 
 \cite{OlssonG:02} related to \cite{GrundyHM:98}, seems to be a concrete instantiation; automatically derives traceabilities from fixed meta-models; if these are broken, automatically propagates updates when possible, or warns the user; all hard-coded.

 \cite{EramoPRV:08} propose the use of ASP to keep multi-view frameworks consistent; many-to-many correspondences are defined between elements, which are used to propagate updates; state-based, operations are derived from the difference between pre- and post-state; a set of changes is proposed to the user, which selects one. these changes simply map operations on elements on modification on other possibly transitively affected elements (e.g., modifying an element may trigger the modification of the correspondent element, or the modification/removal of the correspondence link; these in turn may trigger other hypothetic affected elements). not stable; not correct; not even partially correct; maybe total if always able to calculate the edit operations from the states. It is interactive in the sense that, when two conflicting propagations are detected, it asks the user which one to follow, and then generates the consequent edits.

 \subsubsection{Manually Specifying Repair Information} \label{sec:xiong}

 % fixing actions
 \cite{XiongHZSTM:09} present an approach that combines the detection of errors with the generation of actions to repair them on UML models. They use their own language to define the consistency relations. This language, called Beanbag, has a syntax similar to \textit{Object Constraint Language} (OCL) and together with the specification of consistency rules, it allows to specify how models breaking such rules should be fixed. Rules can then be run either in checking or fixing mode to repair models. More precisely, Beanbag attaches fixing actions to primitive constraints and functions, and composes them through logic operators and other high-level constructs.

 This approach is completely automatic, i.e., without requiring user interaction. In contrast to this method, there are approaches which generate fixing actions purely from a consistency relation, but require human interventions in executing the actions, by specifying some locations to fix, choosing one among a set of actions or filling some missed parameters. Nevertheless, the authors believe both types of approaches are important to consistency management, because while some consistency relations are suitable to be established all the time through automatic fixing, some are suitable to be manually resolved by humans.

 %scalability and clear semantics 
 As the authors state, compared to \textit{Constraint Satisfaction Problem} (CSP) approaches, Beanbag is a more lightweight approach in the sense that it requires users to describe the fixing behavior in the Beanbag program, and thus does not suffer from the scalability problem. Moreover, they compare Beanbag to heuristics-driven methods claiming their approach provides a more clear, predictable fixing semantics, so that end users can clearly know how their updates affect other parts of the model.
 \subsubsection{Relational Model Finding} \label{sec:straeten}

 \cite{StraetenPM:11} assessed the viability of using Kodkod \cite{torlak2007kodkod} to perform model repair. Kodkod is a SAT-based constraint solver for first order logic with relations, transitive closure, bit-vector arithmetic, and partial models. Kodkod is used as a model finder used in a wide range of applications, including, for instance, code checking, test-case generation, and lightweight analysis of Alloy \cite{jackson2012software} models. Kodkod implements relational bounds, i.e., relational variables of any arity are bounded by sets of tuples. Basically, the upper bound specifies the tuples that a relation may contain, while the lower bound specifies the tuples that it must contain.

 In this approach, a repaired model is found by relaxing the bounds on some entities and associations. More specifically, nodes and edges suspected of causing the inconsistencies are removed from the lower-bound, and the upper-bound is augmented to allow additions. To minimise repairs, they first use an external procedure to identify such potentially guilty model elements. However, this technique does not ensure minimality of the repairs, it only handles one inconsistency at a time, and is still not fully automatised (e.g., the relaxation of upper-bounds is performed manually). The authors claim that, performance wise, Kodkod is not viable for model repair of large size models.

 \subsubsection{Heuristics-driven State-space Exploration} \label{sec:hegedus}

 \cite{HegedusHRBV:11} present an approach that is based on graph transformations which generates quick fixes for \textit{Domain Specific Modelling Languages} (DSMLs). According to the authors, while domain-specific editors are usually capable of ensuring that elementary editing operations preserve syntactic correctness (by e.g. syntax-driven editing), most DSMLs include additional language-specific consistency rules that must also be checked. Their aim is thus to provide a domain-independent framework (that is applicable for a wide range of DSMLs), which can efficiently compute complex fixing action sequences even when multiple, overlapping inconsistency rule violations are present in the model. Thereby, the authors propose to adapt the concept of quick fixes (also called error correction, code completion) found in the programming languages domain to DSMLs.

 To capture inconsistency rules of a DSML, they use graph patterns that define declarative structural constraints. Their technique uses graph transformation rules to specify elementary fix operations (policies). These operations are automatically combined by a structural constraint solving algorithm that relies on heuristics-driven state-space exploration to find quick fix sequences efficiently. The technique guarantees that the number of inconsistencies on the model decreases, even if side-effects occur. This is achieved by applying every candidate fix to the inconsistent model and detecting and counting the inconsistencies in the resulting model. The heuristics-guided algorithm automatically selects the best solutions. The engine is capable of generating solutions for a given local scope independently of the total number of violations in other parts of the model.

% \putbib[IEEEabrv,surv]
% \end{bibunit}
